# Supplementary material for: Vec2Gloss: definition modeling leveraging contextualized vectors with Wordnet gloss
Source: arXiv:2305.17855 source file (2023-05-29)
Supplement: Supplementary file 1 [file appendix.tex]

% appendix

\begin{figure*}
\centering
\includegraphics[width=0.75\textwidth]{images/lex.chunk1.png}
\caption{Annotated chunk type distribution}
\label{fig.chunk.dis}
\end{figure*}

\begin{figure*}
\centering
\includegraphics[width=0.75\textwidth]{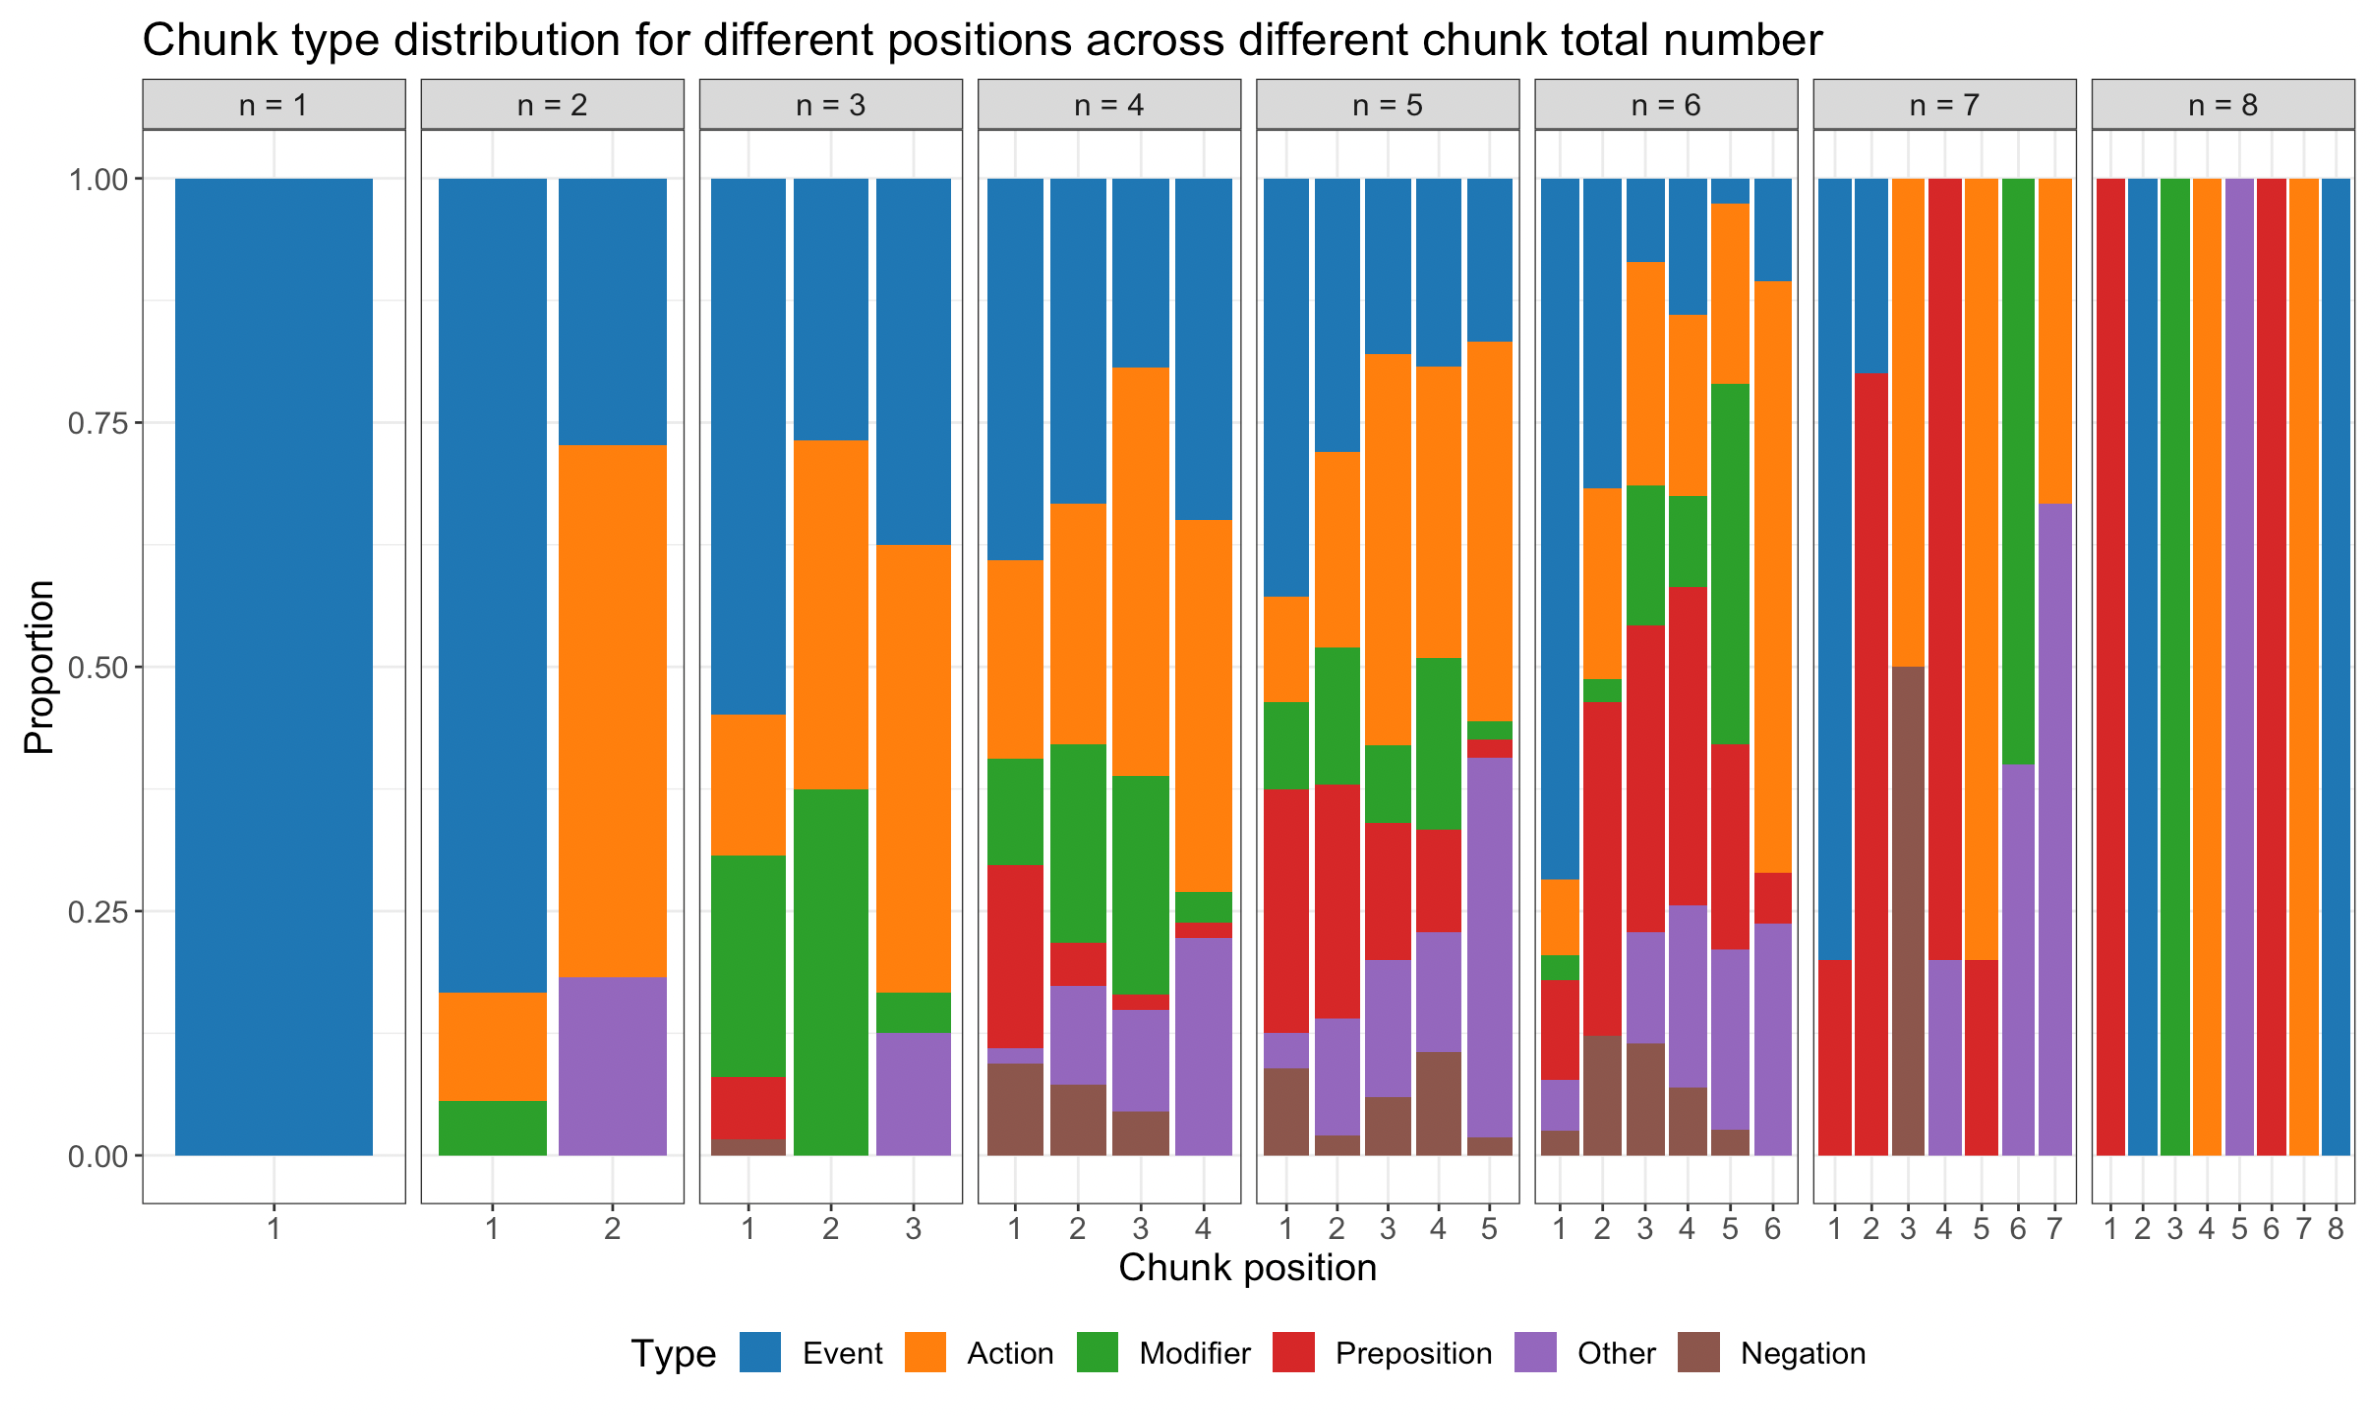}
\caption{Annotated chunk type distribution}
\label{fig.chunk.dis}
\end{figure*}
